# Supplementary material for: A note on metapopulation models
Source: arXiv:2506.04284 ancillary file (2025-06-04)
Supplement: Supplementary file 1 [file A_note_on_metapopulation_models_SM.pdf]

# Supplementary Material for “A note on metapopulation models”

Diepreye Ayabina, Hasan Sevil, Adam Kleczkowski, M. Gabriela M. Gomes

Here we provide extra text and figures referenced in the main text.

## S1 SI model with heterogeneous connectivity

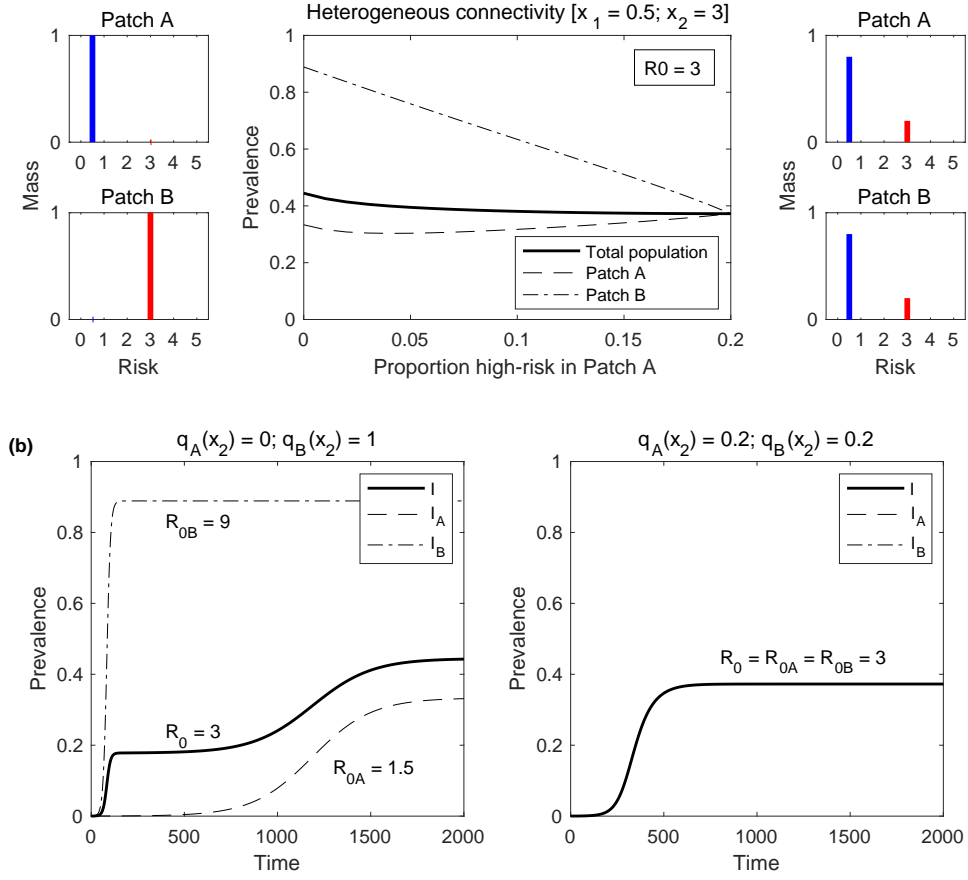

Figure S1: Forward analysis of a SI metapopulation model with heterogeneous connectivity and fixed  $R_0$ . (a) Endemic prevalence as a function of  $q_A(x_2)$ ; (b) Simulated infection growth curves at the lower and higher admissible values for  $q_A(x_2)$ .

## S2 SIR model with heterogeneous connectivity

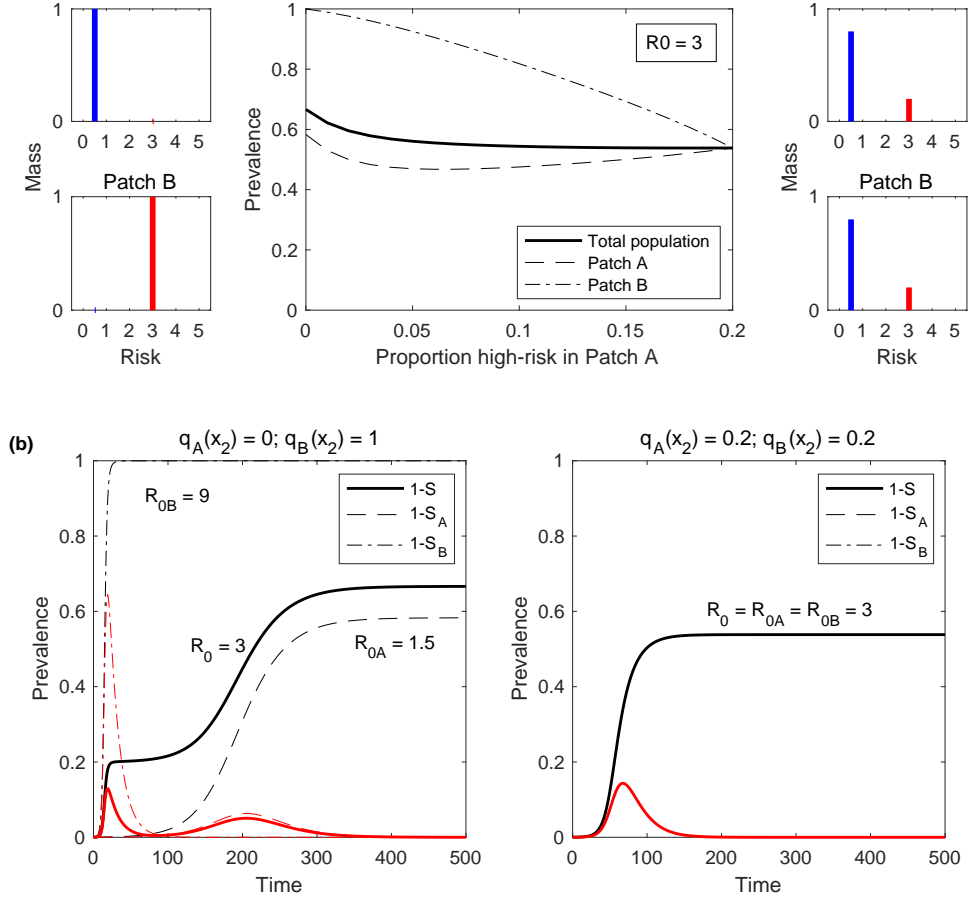

Figure S2: Forward analysis of SIR metapopulation model with heterogeneous connectivity and fixed  $R_0$ . (a) Epidemic final size as a function of  $q_A(x_2)$ ; (b) Simulated infection growth curves at the lower and higher admissible values for  $q_A(x_2)$ .

### S3 SIR model intervention scenarios

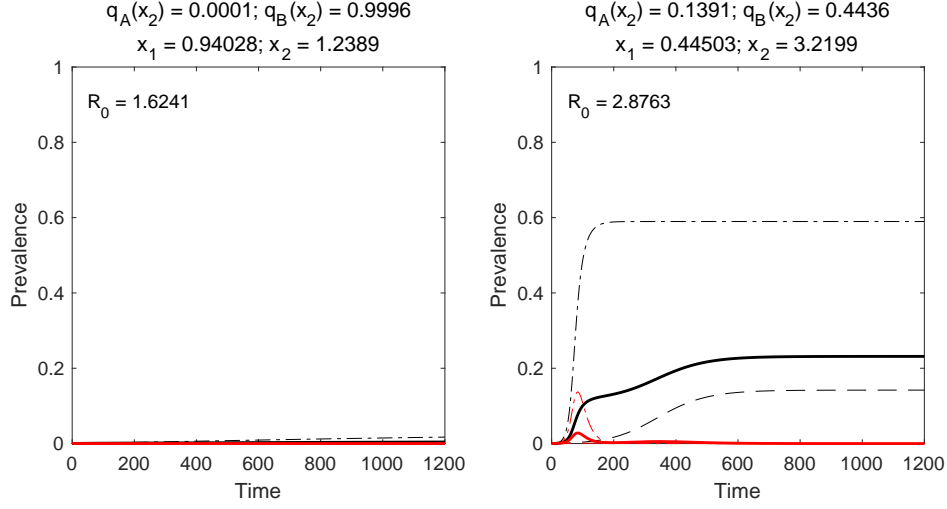

Figure S3: Intervention impact according to SIR metapopulation model with heterogeneous susceptibility. Simulated infection curves of Figure 9(c) modified by an intervention that reduces the susceptibility of all individuals by 50%.

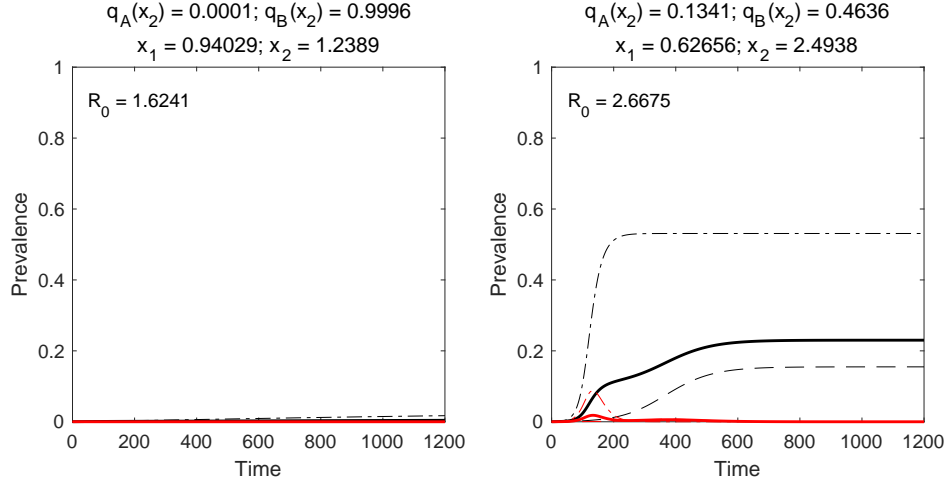

Figure S4: Intervention impact according to SIR metapopulation model with heterogeneous connectivity. Simulated infection curves of Figure 12(c) modified by an intervention that reduces the susceptibility of all individuals by 50%.

### S4 COVID-19 and deprivation

The populations of Aberdeen and Dundee consist of approximately  $N_A = 227,560$  and  $N_B = 147,720$  individuals, respectively. Figure S5 shows visually the data used to inform the epidemic metapopulation models described in Section 2.2 of the main text. The Scottish Index of Multiple Deprivation 2020 (SIMD) plotted on the bottom panels indicate that Aberdeen (Patch A) has a high-risk proportion  $q_A(x_2) = 0.10$  while in Dundee (Patch B) the high-risk proportion is  $q_B(x_2) =$

0.37. The COVID-19 data plotted on the top panels suggest that by October 2023, the ratios of number of cases to population were  $R_A(\infty) = 36\%$  in Aberdeen and  $R_B(\infty) = 40\%$  in Dundee.

To apply the 2-patch SIR metapopulation models to this setting, we derive the low-risk proportions for both patches ( $q_A(x_1) = 1 - q_A(x_2)$  and  $q_B(x_1) = 1 - q_B(x_2)$ ) and write  $x_1$  in terms of  $x_2$  as outlined in Section 2.2 ( $x_1 = (1 - Q(x_2)x_2)/(1 - Q(x_2))$ , where  $Q(x_2) = (q_A(x_2) * N_A + q_B(x_2) * N_B)/(N_A + N_B)$ ). Then we use the Matlab fsolve function to infer  $x_2$  (and subsequently  $x_1$ ) and  $\beta$  (also  $\theta_A$  and  $\theta_B$  when heterogeneity is in connectivity). From these values we then calculate  $\mathcal{R}_0 = 1.25$  and obtain the coefficients of variation for the metapopulation risk distribution as 0.047 when heterogeneity is in susceptibility and 0.045 when heterogeneity is in connectivity.

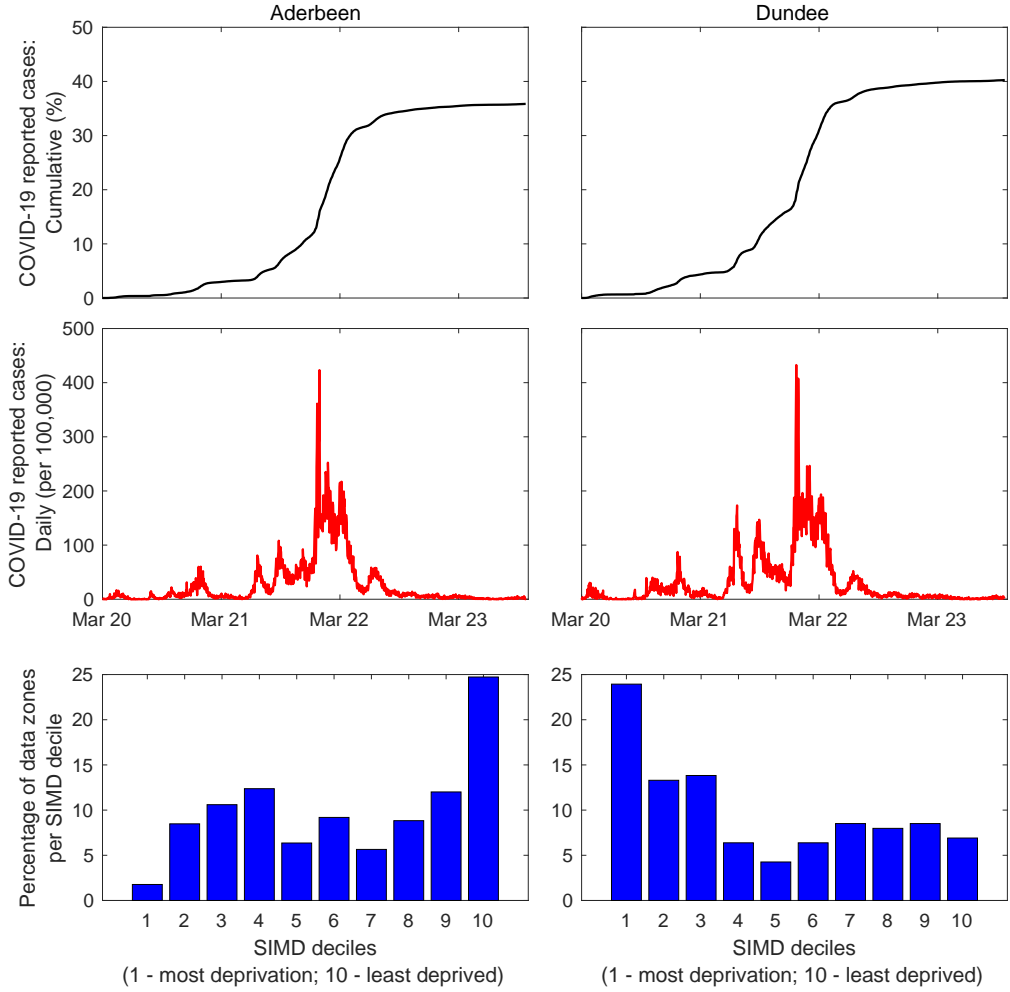

Figure S5: Data for the cities of Aberdeen and Dundee, Scotland. Cumulative COVID-19 reported cases (top). Daily COVID-19 reported cases (middle). Deprivation data according to the Scottish Index of Multiple Deprivation 2020 (bottom).
